# Supplementary material for: Finfluencers on TikTok: A Longitudinal Analysis of Content, Engagement, and Disclaimer Practices
Source: arXiv:2607.05203 source file (2026-07-06)
Supplement: Supplementary file 1 [file appendix.tex]

\appendix
\section{Finance-Related Search Keywords}
\label{sec:finkeywords}
\vspace{-1.5mm}
The finance-related search keywords used for TikTok video retrieval were:
%\begin{lstlisting}
\textquotedblleft budgeting\textquotedblright, \textquotedblleft crypto\textquotedblright, \textquotedblleft cryptocurrency\textquotedblright, \textquotedblleft debtfree\textquotedblright, \textquotedblleft debtpayoff\textquotedblright, \textquotedblleft finance\textquotedblright, 
\textquotedblleft financetiktok\textquotedblright, \textquotedblleft financialeducation\textquotedblright, \textquotedblleft financialfreedom\textquotedblright, \textquotedblleft financialliteracy\textquotedblright, 
\textquotedblleft fintok\textquotedblright, \textquotedblleft investing\textquotedblright, \textquotedblleft investingtips\textquotedblright, \textquotedblleft money\textquotedblright, \textquotedblleft moneygamemoneymindset\textquotedblright, 
\textquotedblleft moneymanagement\textquotedblright, \textquotedblleft moneytok\textquotedblright, \textquotedblleft passiveincome\textquotedblright, \textquotedblleft personalfinance\textquotedblright, 
\textquotedblleft realestateinvesting\textquotedblright, \textquotedblleft retirementplanning\textquotedblright, \textquotedblleft richmindset\textquotedblright, \textquotedblleft savemoney\textquotedblright, 
\textquotedblleft stockmarket\textquotedblright, \textquotedblleft stocks\textquotedblright, \textquotedblleft wealth\textquotedblright, \textquotedblleft wealthbuilding\textquotedblright.

%-----------------------------------------------------------------------------
